# Supplementary material for: Model-Based Reinforcement Learning via Latent-Space Collocation
Source: arXiv:2106.13229 source file (2021-08-07)
Supplement: Supplementary file 1 [file appendix.tex]

\documentclass{article} %
\usepackage{iclr2021_conference,times}

\usepackage{hyperref}
\usepackage{url}
\usepackage{booktabs}       %
\usepackage{amsfonts}       %
\usepackage{nicefrac}       %
\usepackage{microtype}      %

\usepackage{amsfonts, amsmath}
\usepackage{tikz}
\usepackage{pgf}
\usepackage{enumitem}
\usepackage{mathtools}
\usepackage{bbm}
\usepackage{graphicx}
\usepackage{enumitem}
\usepackage{amsthm,amssymb}
\usepackage{amssymb}
\usepackage{booktabs}
\usepackage{float}
\usepackage{wrapfig}
\usepackage{caption} 
\usepackage{ulem}
\usepackage{xspace}
\usepackage{algorithm}
\usepackage[noend]{algorithmic}
\usepackage{caption}
\usepackage{subcaption}

\input{math_commands.tex}

\usepackage{tikz}

\title{Supplemental Material: \\ MBRL via Latent-Space Collocation}

\author{Antiquus S.~Hippocampus, Natalia Cerebro \& Amelie P. Amygdale \thanks{ Use footnote for providing further information
about author (webpage, alternative address)---\emph{not} for acknowledging
funding agencies.  Funding acknowledgements go at the end of the paper.} \\
Department of Computer Science\\
Cranberry-Lemon University\\
Pittsburgh, PA 15213, USA \\
\texttt{\{hippo,brain,jen\}@cs.cranberry-lemon.edu} \\
\And
Ji Q. Ren \& Yevgeny LeNet \\
Department of Computational Neuroscience \\
University of the Witwatersrand \\
Joburg, South Africa \\
\texttt{\{robot,net\}@wits.ac.za} \\
\AND
Coauthor \\
Affiliation \\
Address \\
\texttt{email}
}

\begin{document}

\maketitle

\appendix
\input{sections/06_appendix}

\bibliography{bibtex,bibref_definitions_long}
\bibliographystyle{iclr2021_conference}

\end{document}
